# Supplementary material for: Synthesizing Invariants for Polynomial Programs by Semidefinite Programming
Source: arXiv:2310.11133 source file (2024-09-19)
Supplement: Supplementary file 1 [file appendix.tex]

\newpage
\section{Appendix}
\label{sec:app}

\subsection{Binary Search Strategy} 
\label{app:search}

In the binary search scheme, we start with an initial partition $C_{\bm{a}} = C'_{\bm{a}} \cup C''_{\bm{a}}$, where $C'_{\bm{a}}$ and $C''_{\bm{a}}$ are disjoint.
It is straight forward to see that the valid set $R_I$ w.r.t. $C_{\bm{a}}$ 
is the union of the valid set $R'_I$ and $R''_I$ w.r.t. $C'_{\bm{a}}$ and $C''_{\bm{a}}$ respectively.
Therefore, under-approximations of $R_I$ can be obtained by 
taking the union of under-approximations of $R'_I$ and $R''_I$. 
%One may therefore design a simple recursive procedure accordingly. 
Notice that the objective value of Prog.~(\ref{eq:qsos-inv-relax}), denoted by $v$, is actually the rescaled integral of the polynomial $h_{d}(\bm{a})$ over $C_{\bm{a}}$. 
As $h_{d}(\bm{a})$ approximates $J(\bm{a})$ from the above, 
the optimal value $v$ measures the approximation gap to some extent. 
Furthermore, since a feasible approximation $h_{d}(\bm{a})$ over $C_{\bm{a}}$ is still feasible over $C'_a$ and $C''_a$, 
there will always be $\Delta v = v - \frac{1}{2} (v' + v'') \geq 0$, where $v'$ and $v''$ are the respective objective values obtained by solving Prog.~(\ref{eq:qsos-inv-relax}) over $C'_{\bm{a}}$ and $C''_{\bm{a}}$.
Consequently, one may use the difference $\Delta v$ to measure the improvements induced by each partitioning step. 
The binary search scheme stops either when the size of the current $C_{\bm{a}}$ becomes sufficiently small or when the improvement $\Delta v$ is below a predefined threshold.
The overall scheme is summarized as Algorithm~\ref{alg:adp}.

Unfortunately, we have observed that the binary search framework for the Cluter algorithm can be susceptible to numerical errors when dealing with particularly small parameter domains $C_{\bm{a}}$. 
This limitation necessitates careful tuning of the algorithm's hyper-parameters to ensure successful application. 
We acknowledge this as a potential avenue for future investigation to improve the robustness of the approach.

% Unfortunately, we have found that the binary search framework may fail due to numerical errors when the region of parameters $\bm{a}$ is small.
% To make it work, one need to fine-tune the hyper-parameters in the algorithm.
% We plan to address this problem in future studies.
% experiments have shown that the binary search framework may fail due to numerical errors when the region of parameters $\bm{a}$ is small, and hence requiring fine-tunning techniques. 
% We plan to 

\IncMargin{1em}
\begin{algorithm2e}[h]
\SetKwInOut{Input}{Input}
\SetKwInOut{Output}{Output}
\ResetInOut{Output} 
\Input{
    a hyper-rectangle $C_{\bm{a}}\subseteq \mathbb R^{n'}$
    and thresholds $\epsilon_d,\epsilon_v>0$}
\Output{a polynomial $h\in \mathbb R[\bm{a}]$}
\BlankLine
$C\gets C_{\bm{a}}$\;
$(v,h)\gets$ Solve Prog.~(\ref{eq:qsos-inv-relax}) with respect to $C$
\algocomment*[l]{$v$: optimal value; $h$: polynomial $h_{d}(\bm{a})$}
\While(\algocomment*[h]{$\textsf{Diameter}$ returns the length of the longest side})
{$\textsf{Diameter}(C)>\epsilon_d$}
{
    $(C_{l},C_{r})\gets \textsf{Bisection}(C)$
    \algocomment*[l]{$\textsf{Bisection}$ bisects the rectangle from the longest side}
    $(v_{l},h_{l})\gets$ Solve Prog.~(\ref{eq:qsos-inv-relax}) with respect to $C_l$\;
    $(v_{r},h_{r})\gets$ Solve Prog.~(\ref{eq:qsos-inv-relax}) with respect to $C_r$\;
    $\Delta v = v - \frac{1}{2}(v_l+v_r)$\;
    \lIf(\algocomment*[h]{stop when the improvement is small}){$\Delta v< \epsilon_v$}{break} 
    \eIf{$v_l<v_r$}
    {$(C,v,p)\gets (C_l,v_l,h_l)$\;}
    {$(C,v,p)\gets (C_r,v_r,h_r)$\;}
}
\KwRet{$h$}
\caption{Binary Search}
\label{alg:adp}
\end{algorithm2e}
\DecMargin{1em}

\subsection{Sum-k-Power-d Benchmark}
\label{app:sumpower}
This is a manually constructed example with no practical meanings, solely intended to demonstrate how the number of parameters will influence the efficiency of our algorithm.
It is easy to see $n_{\bm{a}}=\binom{k+d}{d}$.

\begin{listing}[ht]
\begin{minted}[mathescape, escapeinside=||]{c}
    // Program variables: $(n_1,n_2,\dots,n_k,s)\in \Real^n$
    // Precondition: $s=(n_1+n_2+\dots+n_k)^d$
    // Invariant template: {$s= {\color{purple} poly[(n_1,\dots,n_k),d]}$}
    while ( true ) { // Real invariant $s=(n_1+n_2+\dots+n_k)^d$
        |$n_1 = n_1 + 1$|;
        |$\dots$|;
        |$n_k = n_k + 1$|;
        |$s = (n_1+n_2+\dots+n_k+k)^d - (n_1+n_2+\dots+n_k)^d$|;
    }
    // Postcondition: true
\end{minted}
\caption{\textsf{sum-$k$-power-$d$}}
\label{code:sumpower}
\end{listing}

% \subsection{Mitigating Numerical Errors}
% \label{app:numerical}
